# Supplementary material for: Communication-Efficient Decentralized Online Continuous DR-Submodular Maximization
Source: arXiv:2208.08681 source file (2022-08-18)
Supplement: Supplementary file 1 [file Appendix0.tex]

\begin{lemma}
Let $\{a_{t}\}_{t=0}^{K}$ be a sequence of points in $\R^{n}$ such that $\|a_{t}-a_{t-1}\|\le\frac{G}{K+s-t}$ for all $1\le t\le K$ with fixed constant $G\ge0$ and $s\ge 2$. Let $\{\widetilde{a}_{t}\}_{t=0}^{K}$ be a sequence of random variables such that $\E(\widetilde{a}_{t}|\F_{t-1})=a_{t}$ and $\E(\|\widetilde{a}_{t}-a_{t}\|^{2}|\F_{t-1})\le\sigma^{2}$ for every $t\ge0$, where $\F_{t-1}$ is the $\sigma$-field generated by $\{\widetilde{a}_{t}\}_{t=0}^{K}$ and $\F_{0}=\emptyset$. Let $\{d_{t}\}_{t=0}^{K}$ be a sequence of random variables where $d_{0}$ is fixed and subsequent $d_{t}$ are obtained by $d_{t}=(1-\eta_{t})d_{t-1}+\eta_{t}\widetilde{a}_{t}$. If we set $\eta_{t}=\frac{2}{(t+3)^{2/3}}$, when $1\le t\le\lfloor\frac{K+s}{2}\rfloor$, and when $\lfloor\frac{K+s}{2}\rfloor+1\le t\le K$, $\eta_{t}=\frac{1.5}{(K-t+s)^{2/3}}$, we have
\begin{equation}
    \E(\|d_{t}-a_{t}\|^{2})\le\left\{\begin{aligned}
       &\frac{N}{(t+4)^{2/3}}& 1\le t\le\lfloor\frac{K+s}{2}\rfloor\\
       &\frac{N}{(K+s-t-1)^{2/3}}& \lfloor\frac{K+s}{2}\rfloor+1\le t\le K
    \end{aligned}\right.
\end{equation} where $N=\max\{5^{2/3}\|a_{0}-d_{0}\|^{2},4\sigma^{2}+32G,2.25\sigma^{2}+7G/3\}$.
\end{lemma}
\begin{proof}
\begin{equation}
\begin{aligned}
   \|d_{t}-a_{t}\|^{2}&=\|(1-\eta_{t})d_{t-1}+\eta_{t}\widetilde{a}_{t}-a_{t}\|\\
   &=\|(1-\eta_{t})(d_{t-1}-a_{t-1})+(1-\eta_{t})(a_{t-1}-a_{t})+\eta_{t}(\widetilde{a}_{t}-a_{t})\|^{2}\\
   &=(1-\eta_{t})^{2}\|d_{t-1}-a_{t-1}\|^{2}+(1-\eta_{t})^{2}\|a_{t-1}-a_{t}\|^{2}+\eta_{t}^{2}\|\widetilde{a}_{t}-a_{t}\|^{2}\\
   &+2(1-\eta_{t})^{2}\langle d_{t-1}-a_{t-1}, a_{t-1}-a_{t}\rangle+2(1-\eta_{t})\eta_{t}\langle d_{t-1}-a_{t-1}, \widetilde{a}_{t}-a_{t}\rangle\\
   &+2(1-\eta_{t})\eta_{t}\langle a_{t-1}-a_{t}, \widetilde{a}_{t}-a_{t}\rangle.
\end{aligned}
\end{equation}
Also, we could get
\begin{equation}
    \begin{aligned}
       \E(\langle d_{t-1}-a_{t-1}, \widetilde{a}_{t}-a_{t}\rangle)&= \E(\E(\langle d_{t-1}-a_{t-1}, \widetilde{a}_{t}-a_{t}\rangle)|\F_{t-1})\\
       &=\E(\E(\langle d_{t-1}-a_{t-1}, \E(\widetilde{a}_{t}|\F_{t-1})-a_{t}\rangle)=0.
    \end{aligned}
\end{equation}
\begin{equation}
    \begin{aligned}
       \E(\langle a_{t-1}-a_{t}, \widetilde{a}_{t}-a_{t}\rangle)&= \E(\E(\langle a_{t-1}-a_{t}, \widetilde{a}_{t}-a_{t}\rangle)|\F_{t-1})\\
       &=\E(\E(\langle a_{t-1}-a_{t}, \E(\widetilde{a}_{t}|\F_{t-1})-a_{t}\rangle)=0.
    \end{aligned}
\end{equation}
Therefore, we have 
\begin{equation}
    \begin{aligned}
    \E(\|d_{t}-a_{t}\|^{2})&=(1-\eta_{t})^{2}\E(\|d_{t-1}-a_{t-1}\|^{2})+(1-\eta_{t})^{2}\E(\|a_{t-1}-a_{t}\|^{2})+\eta_{t}^{2}\E(\|\widetilde{a}_{t}-a_{t}\|^{2})\\
   &+2(1-\eta_{t})^{2}\E(\langle d_{t-1}-a_{t-1}, a_{t-1}-a_{t}\rangle)\\
   &\le(1-\eta_{t})^{2}\E(\|d_{t-1}-a_{t-1}\|^{2})+(1-\eta_{t})^{2}\E(\|a_{t-1}-a_{t}\|^{2})+\eta_{t}^{2}\E(\|\widetilde{a}_{t}-a_{t}\|^{2})\\
   &+(1-\eta_{t})^{2}\frac{\eta_{t}}{2}\E(\|d_{t-1}-a_{t-1}\|^{2})+(1-\eta_{t})^{2}\frac{2}{\eta_{t}}\E(\|a_{t-1}-a_{t}\|^{2})\\
   &\le(1-\eta_{t})^{2}(1+\frac{\eta_{t}}{2})\E(\|d_{t-1}-a_{t-1}\|^{2})+(1-\eta_{t})^{2}(1+\frac{2}{\eta_{t}})\E(\|a_{t-1}-a_{t}\|^{2})+\eta_{t}^{2}\sigma^{2}\\
   &\le(1-\eta_{t})\E(\|d_{t-1}-a_{t-1}\|^{2})+(1+\frac{2}{\eta_{t}})\E(\|a_{t-1}-a_{t}\|^{2})+\eta_{t}^{2}\sigma^{2}\\
   &\le(1-\eta_{t})\E(\|d_{t-1}-a_{t-1}\|^{2})+(1+\frac{2}{\eta_{t}})\frac{G}{(K+s-t)^{2}}+\eta_{t}^{2}\sigma^{2}.
    \end{aligned}
\end{equation}
If we set $\triangle_{t}=\E(\|d_{t}-a_{t}\|^{2})$, we have
\begin{equation}
    \triangle_{t}\le(1-\eta_{t})\triangle_{t-1}+(1+\frac{2}{\eta_{t}})\frac{G}{(K+s-t)^{2}}+\eta_{t}^{2}\sigma^{2}.
\end{equation}
When $1\le t\le\lfloor\frac{K+s}{2}\rfloor$, we have 
\begin{equation}
    \begin{aligned}
    \triangle_{t}&\le(1-\frac{2}{(t+3)^{2/3}})\triangle_{t-1}+(1+(t+3)^{2/3})\frac{G}{(K+s-t)^{2}}+\frac{4\sigma^{2}}{(t+3)^{4/3}}\\
    &\le(1-\frac{2}{(t+3)^{2/3}})\triangle_{t-1}+(1+(t+3)^{2/3})\frac{G}{t^{2}}+\frac{4\sigma^{2}}{(t+3)^{4/3}}\\
    &\le(1-\frac{2}{(t+3)^{2/3}})\triangle_{t-1}+(1+(t+3)^{2/3})\frac{G}{(t+3)^{2}}\frac{(t+3)^{2}}{t^{2}}+\frac{4\sigma^{2}}{(t+3)^{4/3}}\\
    &\le(1-\frac{2}{(t+3)^{2/3}})\triangle_{t-1}+(1+(t+3)^{2/3})\frac{16G}{(t+3)^{2}}+\frac{4\sigma^{2}}{(t+3)^{4/3}}\\
    &\le(1-\frac{2}{(t+3)^{2/3}})\triangle_{t-1}+\frac{16G}{(t+3)^{2}}+\frac{4\sigma^{2}+16G}{(t+3)^{4/3}}\\
    &\le(1-\frac{2}{(t+3)^{2/3}})\triangle_{t-1}+\frac{4\sigma^{2}+32G}{(t+3)^{4/3}}\\
    &\le(1-\frac{2}{(t+3)^{2/3}})\triangle_{t-1}+\frac{N}{(t+3)^{4/3}}
    \end{aligned}
\end{equation} where the second inequality comes from $K+s-t\ge t$; the fourth inequality from $\frac{t+3}{t}\le 4$, when $t\ge 1$; the final from $N\ge4\sigma^{2}+32G$. 

Then, we verify that $\triangle_{t}\le\frac{N}{(t+4)^{2/3}}$, where $1\le t\le\lfloor\frac{K+s}{2}\rfloor$. By induction, $\triangle_{1}\le \frac{N}{5^{2/3}}$. If we assume $\triangle_{t-1}\le\frac{N}{(t+3)^{2/3}}$, we have
\begin{equation}\label{equ:22}
    \begin{aligned}
    \triangle_{t}&\le(1-\frac{2}{(t+3)^{2/3}})\triangle_{t-1}+\frac{N}{(t+3)^{4/3}}\\
    &\le(1-\frac{2}{(t+3)^{2/3}})\frac{N}{(t+3)^{2/3}}+\frac{N}{(t+3)^{4/3}}\\
    &\le\frac{N((t+3)^{2/3}-1)}{(t+3)^{4/3}}\\
    &\le\frac{N}{(t+4)^{2/3}},
    \end{aligned}
\end{equation}where the final equality comes from $\frac{(t+3)^{2/3}-1}{(t+3)^{4/3}}\le\frac{1}{(t+4)^{2/3}}$.

When $\lfloor\frac{K+s}{2}\rfloor+1\le t\le K$, here $\eta_{t}=\frac{1.5}{(K+s-t)^{2/3}}$, so we have 
\begin{equation}
    \begin{aligned}
    \triangle_{t}&\le(1-\frac{1.5}{(K+s-t)^{2/3}})\triangle_{t-1}+\frac{2.25\sigma^{2}}{(K+s-t)^{4/3}}+(1+\frac{4}{3}(K+s-t)^{2/3})\frac{G}{(K+s-t)^{2}}\\
    &\le(1-\frac{1.5}{(K+s-t)^{2/3}})\triangle_{t-1}+\frac{2.25\sigma^{2}}{(K+s-t)^{4/3}}+\frac{4G/3}{(K+s-t)^{4/3}}+\frac{G}{(K+s-t)^{2}}\\
    &\le(1-\frac{1.5}{(K+s-t)^{2/3}})\triangle_{t-1}+\frac{2.25\sigma^{2}+7G/3}{(K+s-t)^{4/3}}\\
    &\le(1-\frac{1.5}{(K+s-t)^{2/3}})\triangle_{t-1}+\frac{N}{(K+s-t)^{4/3}}.
    \end{aligned}
\end{equation}
When $t=\lfloor\frac{K+s}{2}\rfloor$, according to \ref{equ:22}, we have
\begin{equation}
    \triangle_{\lfloor\frac{K+s}{2}\rfloor}\le \frac{N}{(\lfloor\frac{K+s}{2}\rfloor+4)^{2/3}}\le\frac{N}{(K+s-\lfloor\frac{K+s}{2}\rfloor-1)^{2/3}},
\end{equation} where $K+s-\lfloor\frac{K+s}{2}\rfloor-1\le\lfloor\frac{K+s}{2}\rfloor+4$.
By induction, we assume $\triangle_{t-1}\le\frac{N}{K+s-t}$, then 
\begin{equation}
    \begin{aligned}
    \triangle_{t}\le\frac{N((K+s-t)^{2/3}-0.5)}{(K+s-t)^{4/3}}\le\frac{N}{(K+s-t-1)^{2/3}},
    \end{aligned} 
\end{equation}where $\frac{(K+s-t)^{2/3}-0.5}{(K+s-t)^{4/3}}\le\frac{1}{(K+s-t-1)^{2/3}}$.
\end{proof}

 &\le\dots\\
    &\le(1-\gamma)^{s}NG+(1-\gamma)\sum_{m=1}^{s}(1-\gamma)^{s-m}\frac{N(2G+LR)}{K-m+2}\\
    &+\gamma\sum_{m=1}^{s}(1-\gamma)^{s-m}\|\sum_{i=1}^{N}g_{i}^{(m)}(q)
    -\sum_{i=1}^{N}\nabla\bar{f}_{i,q,m}(x_{i}^{(m)}(q))\|+\frac{LNR}{K(1-\beta)}
